# Supplementary material for: Quantifying and controlling the magnetic dipole contribution to 1.5 $\mu$m light emission in erbium-doped yttrium oxide
Source: arXiv:1402.3717 ancillary file (2014-02-15)
Supplement: Supplementary file 1 [file DLi_ErY2O3_SuppMat.pdf]

## *Supplemental Material:* Quantifying and controlling the magnetic dipole contribution to 1.5 $\mu$m light emission in erbium-doped yttrium oxide

Dongfang Li,[1,2] Mingming Jiang,[1,2] Sébastien Cueff,[1,*]
Christopher M. Dodson,[1] Sinan Karaveli,[1,†] and Rashid Zia[1,2,‡]

[1]*School of Engineering, Brown University, Providence, RI 02912, USA*
[2]*Department of Physics, Brown University, Providence, RI 02912, USA*
(Dated: February 15, 2014)

## Emission rate and spectral analysis

To predict the observed far-field emission spectra as a function of the emitter-mirror separation distance ($d$), we combine a three-layer model for the LDOS [1–3] with the spectrally resolved intrinsic emission rates ($\Gamma_0^{ED}(\lambda)$ and $\Gamma_0^{MD}(\lambda)$) measured by energy-momentum spectroscopy [4]. The ED and MD emission rates as a function of wavelength and separation distance ($\Gamma^{ED}(\lambda,d)$ and $\Gamma^{MD}(\lambda,d)$) can be calculated through Eqs. (S1) and (S2) [1, 2], respectively.

$$\frac{\Gamma^{ED}}{\Gamma_0^{ED}}=\tilde{\rho}^{ED}=\frac{1}{2}\,\mathrm{Im}\left[\int_0^{u_{\max}}\left(\frac{(1+R_{12}^s)(1+R_{13}^s)}{1-R_{12}^sR_{13}^s}+\frac{(1+R_{12}^p)(1+R_{13}^p)-2u^2(R_{12}^p+R_{13}^p)}{1-R_{12}^pR_{13}^p}\right)\frac{udu}{l_1}\right], \qquad \text{(S1)}$$

$$\frac{\Gamma^{MD}}{\Gamma_0^{MD}}=\tilde{\rho}^{MD}=\frac{1}{2}\,\mathrm{Im}\left[\int_0^{u_{\max}}\left(\frac{(1-R_{12}^p)(1-R_{13}^p)}{1-R_{12}^pR_{13}^p}+\frac{(1-R_{12}^s)(1-R_{13}^s)+2u^2(R_{12}^s+R_{13}^s)}{1-R_{12}^sR_{13}^s}\right)\frac{udu}{l_1}\right], \qquad \text{(S2)}$$

where the subscript 1 stands for the combined $Y_2O_3$ emitter and spacer layer, 2 is the quartz substrate, and 3 represents the gold mirror whose refractive index is approximated using the Lorentz-Drude model [5]. $R_{ij}^{s,p}=r_{ij}^{s,p}e^{-2kl_is_{ij}}$ is the reflection coefficient for the reflected electric field from the gold mirror, $r_{ij}^s=(l_i-l_j)/(l_i+l_j)$ and $r_{ij}^p=(\varepsilon_il_j-\varepsilon_jl_i)/(\varepsilon_il_j+\varepsilon_jl_i)$ are the reflection coefficients for s- and p-polarization. The distance from the emitters to the quartz substrate $s_{12}$ is fixed to be 109 nm (the thickness of the bottom buffer layer plus half of the emitter layer thickness), whereas the separation distance between emitters and the gold mirror $s_{13}$ varies from 38 to 735 nm (half of the emitter layer thickness plus the total coating layer thickness). $l_j=-i\sqrt{\varepsilon_j/\varepsilon_1-u^2}$ and $u=k_{||}/k$ are the perpendicular and parallel components of the wave vectors normalized to $k=2\pi n_1/\lambda$. The value of $u_{\max}=NA/\sqrt{\varepsilon_1}$ is set by the objective′s numerical aperture (NA) and the dielectric constant of the emitter host. Since the emission intensity $I(\lambda,d)$ is proportional to the total emission rate $\Gamma(\lambda,d)=\Gamma^{ED}(\lambda,d)+\Gamma^{MD}(\lambda,d)$, the normalized intensity spectra $I_N(\lambda,d)$ can be expressed as:

$$I_N(\lambda,d)=\frac{I(\lambda,d)}{\int I(\lambda,d)d\lambda}=\frac{\Gamma(\lambda,d)}{\int\Gamma(\lambda,d)d\lambda}. \qquad \text{(S3)}$$

For comparison, we also consider an ED only model in which we assume that all emission originates from ED transitions. For this case, using Eqs. (S1) and (S3), we infer the spectrally resolved ED intrinsic emission rates from the normalized intensity spectrum of the original emitter layer sample, as previously described in Ref. 2. Then the theoretical spectra for the ED only model can be predicted using Eqs. (S1) and (S3) [2, 3]. The predictions of the ED only model are shown in Fig. S2 together with the experimental results and the predictions of the combined ED and MD model described above.

[1] R. R. Chance, A. Prock, and R. Silbey, Adv. Chem. Phys. **37**, 1 (1978).
[2] S. Karaveli and R. Zia, Phys. Rev. Lett. **106**, 193004 (2011).
[3] S. Karaveli, A. J. Weinstein, and R. Zia, Nano Lett. **13**, 2264 (2013).
[4] T. H. Taminiau, S. Karaveli, N. F. van Hulst, and R. Zia, Nat. Commun. **3**, 979 (2012).
[5] A. D. Rakic, A. B. Djurišic, J. M. Elazar, and M. L. Majewski, Appl. Opt. **37**, 5271 (1998).
[6] Y. Mao, T. Tran, X. Guo, J. Y. Huang, C. K. Shih, K. L. Wang, and J. P. Chang, Adv. Funct. Mater. **19**, 748 (2009).

*Present address: Institut des Nanotechnologies de Lyon, Ecole Centrale de Lyon, 69134 Ecully, France
†Present address: Research Laboratory of Electronics, Massachusetts Institute of Technology, Cambridge, MA 02139, USA
‡Electronic address: Rashid_Zia@brown.edu

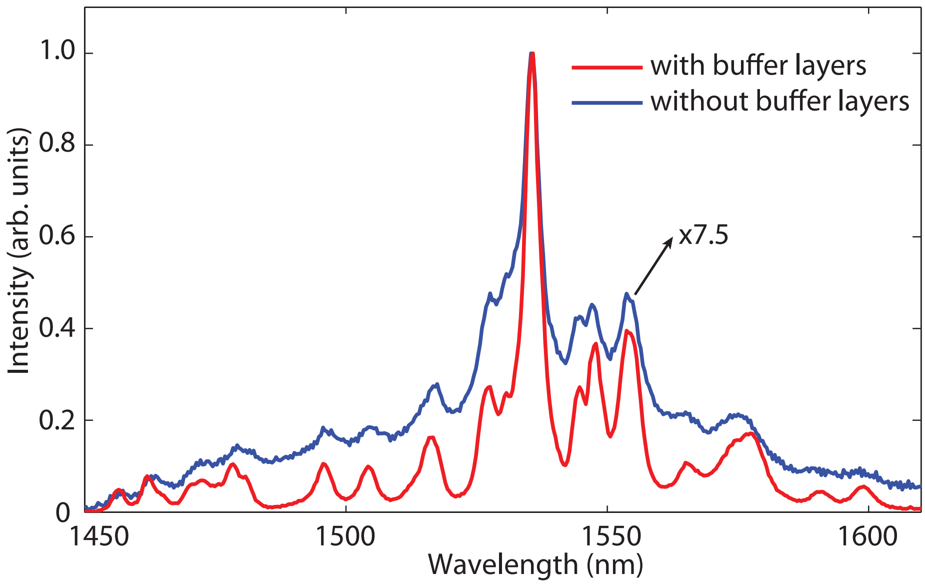


FIG. S1: (Color) Comparison of the emission spectra for the $Er^{3+}$:$Y_2O_3$ layers fabricated with and without pure yttria buffer layers. Both spectra have been normalized to their peak value, but in relative terms, the peak emission of the sample with buffer layers (red line) was ∼7.5 times stronger than that from the sample without buffer layers (blue line). Thus, the sample with buffer layers shows both stronger luminescence and more clearly defined emission peaks, which are indicative of less inhomogeneous broadening. The spectral shape of the sample with buffer layers (red line) is also similar to the luminescence spectrum of low concentration (1 at.%) nanocrystalline erbium-doped yttria (see Fig. 3(d) in Ref. 6).

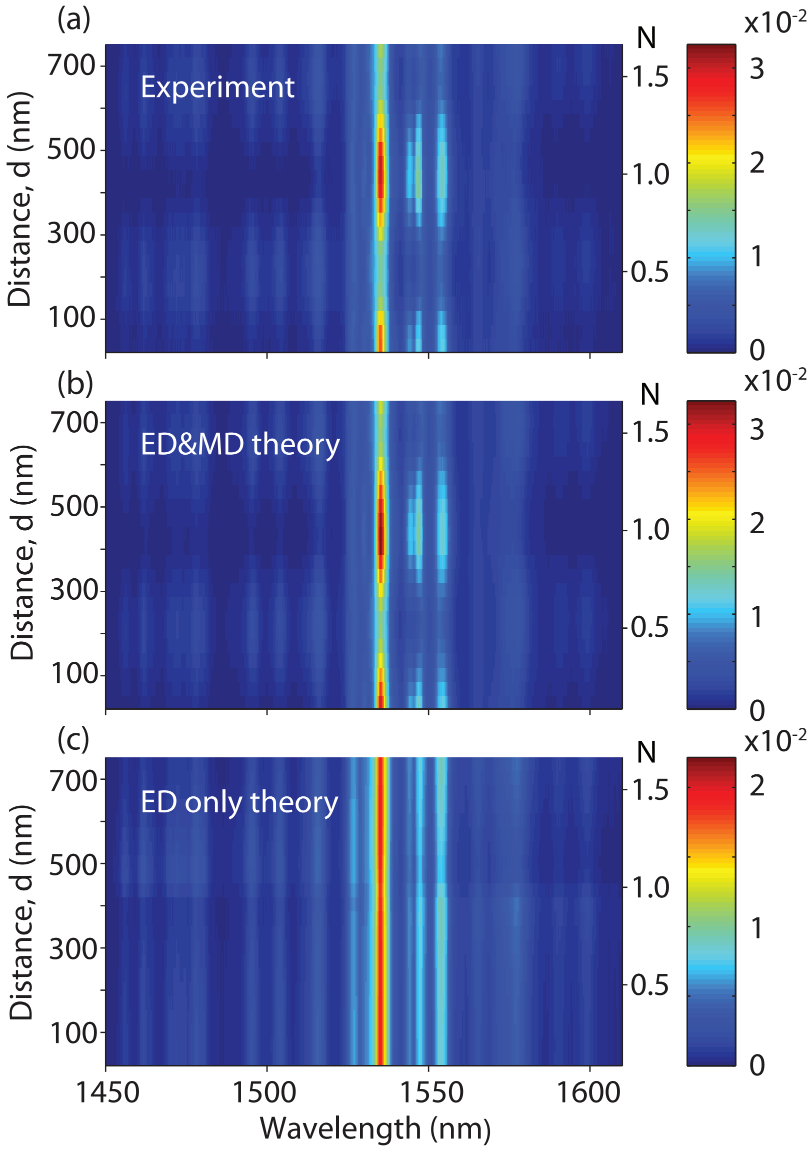


FIG. S2: (Color) (a) Normalized experimental spectra measured for different emitter-mirror separation distances, *d*; each spectra is normalized to its total integrated intensity. (b) Normalized theoretical spectra predicted using the intrinsic ED and MD emission rates from Fig. 1(c) together with the three-layer LDOS model described by Eqs. (S1)-(S3). (c) Normalized theoretical spectra predicted by ED only model. Note that panels (a) and (b) here are identical to Figs. 2(a) and 2(b) in the main text.
